# Supplementary material for: Two-step nucleation of the Earth's inner core
Source: arXiv:2105.07296 source file (2022-01-08)
Supplement: Supplementary file 1 [file SI_v9.pdf]

**Supplementary Information**

# Two-step nucleation of the Earth's inner core

Yang Sun[1], Feng Zhang[2], Mikhail I. Mendelev[2], Renata M. Wentzcovitch[1,3,4], Kai-Ming Ho[5]

[1]Department of Applied Physics and Applied Mathematics, Columbia University, New York, NY 10027, USA
[2]Ames Laboratory, US Department of Energy, Ames, IA 50011, USA
[3]Department of Earth and Environmental Sciences, Columbia University, New York, NY 10027, USA
[4]Lamont–Doherty Earth Observatory, Columbia University, Palisades, NY 10964, USA
[5]Department of Physics, Iowa State University, Ames, IA 50011, USA

Correspondence to ys3339@columbia.edu (Y.S.) or mikhail.mendelev@gmail.com (M.I.M.)

This supplementary information contains details of semi-empirical potential development in Note S1, the calculation of the kinetic prefactor in Note S2, the effect of input parameters on the hcp waiting time in Note S3, and classification of hcp, bcc, and liquid with order parameters in Note S4.

**Supplementary Note 1 | Development of semi-empirical potential**

Several groups of target properties were used in the development of the embedded atom method (EAM) potential for iron. The first group consisted of basic bcc Fe properties at T=0 and p=0 listed in Table S1. This is a standard set routinely used in development procedures for semi-empirical potentials. Since the condition of T=0 and p=0 is very far from the conditions we were interested in, these properties were fitted with low weights. The examination of Table S1 shows that the developed potential reproduces these properties reasonably well (obviously, the semi-empirical potentials explicitly fitted to these conditions provide much better reproduction of these properties).

**Table S1 | Fe bcc properties at T=0 and p=0.**

| Property | Target value | EAM potential |
|---|---|---|
| Lattice parameter (Å) | 2.855 | 2.844 |
| Cohesive energy (eV/atom) | -4.316 | -4.022 |
| Unrelaxed vacancy formation energy (eV/atom) | 1.84 | 1.53 |
| $C_{11}$ (GPa) | 243 | 246 |
| $C_{12}$ (GPa) | 145 | 141 |
| $C_{44}$ (GPa) | 116 | 103 |

Next, we approximately extracted from the *ab initio* molecular dynamics (AIMD) simulation the hcp lattice parameters at two endpoints of the temperature-pressure range we were interested in (T=4000 K/p=140 GPa and T=6000 K/p=350 GPa). This was done by manually adjusting the hcp lattice parameters at these conditions. The accuracy of such a procedure was not very high such that the difference between $\sigma_{xx}$ and $\sigma_{zz}$ could be as significant as 14 GPa. Fortunately, that was not the problem with our fitting procedure. In reality, the potential was fitted not to the lattice parameters but to the stresses corresponding to the given lattice parameters. These stresses were determined from the AIMD simulation with sufficient accuracy. We will come back to this point below. After a few iterations of the potential development procedure, we used the current potential to determine the lattice parameters at T=5500 K/p=212 GPa. We ran AIMD to determine the stresses corresponding to these lattice parameters. In this case, the difference between $\sigma_{xx}$ and $\sigma_{zz}$ were less than 1 GPa. The new data were added to the list of target properties in the potential development procedure. We also included the same type of AIMD data for the bcc phase at T=6000 K/p=350 GPa (in this case, there is just one lattice parameter to fit).

**Table S2 | The elastic response tensors between AIMD and MD with EAM potential.**

| Conditions | Tensor components (GPa) | AIMD | EAM |
|---|---|---|---|
| hcp at T=4000 K p=140 GPa | $R_{11}$ | 820 | 758 |
| | $R_{12}$ | 589 | 614 |
| | $R_{13}$ | 389 | 467 |
| | $R_{33}$ | 832 | 810 |
| | $R_{44}$ | 122 | 105 |
| hcp at T=5500 K p=212 GPa | $R_{11}$ | 1064 | 1015 |
| | $R_{12}$ | 784 | 860 |
| | $R_{13}$ | 671 | 740 |
| | $R_{33}$ | 1185 | 1229 |
| | $R_{44}$ | 122 | 131 |
| hcp at T=6000 K p=350 GPa | $R_{11}$ | 1646 | 1548 |
| | $R_{12}$ | 1235 | 1286 |
| | $R_{13}$ | 1009 | 1142 |
| | $R_{33}$ | 1758 | 1834 |
| | $R_{44}$ | 216 | 203 |
| bcc at T=6000 K p=350 GPa | $R_{11}$ | 1318 | 1291 |
| | $R_{12}$ | 1236 | 1229 |
| | $R_{44}$ | 287 | 307 |

Three types of deformation were applied to each of the hcp models to get non-zero $\varepsilon_{xx}$, $\varepsilon_{zz}$, and $\varepsilon_{yz}$ (the absolute values of $\varepsilon_{\alpha\beta}$ were 0.01). The stress tensor components were determined from the AIMD simulation for each case. The differences between these stress tensor components and the components of the stress tensors of the corresponding initial models divided by the deformation value were defined as the elastic responses, $R_{ij}$. $R_{ij}$ would be the same as the corresponding elastic constants if all components of the stress tensor of the initial model were zero. $R_{ij}$ constants reflect the crystal response to the applied deformation. A good fitting to these constants should warrant the reproduction of the correct elastic properties of the considered phases. The obtained AIMD values are presented in Table S2. It is important to emphasize that the bcc phase did not transform

to any other lattice under applied deformation during the AIMD simulation, demonstrating that this phase is at least metastable (not unstable) at these conditions. The examination of Table S2 shows that the developed potential reasonably well reproduces the elastic responses obtained from the AIMD simulation.

Since we were interested in simulating nucleation from the liquid phase, it is essential to include the liquid density and structure data obtained from the AIMD simulation in the potential development procedure. The method to achieve this was described in [1]. Figure S1 shows the pair correlation functions of liquid Fe obtained from the AIMD simulation and classical MD (CMD) simulation at Earth's core conditions utilizing the developed EAM potential. Examination of this figure indicates that the developed potential provides a pretty reasonable agreement with the AIMD data.

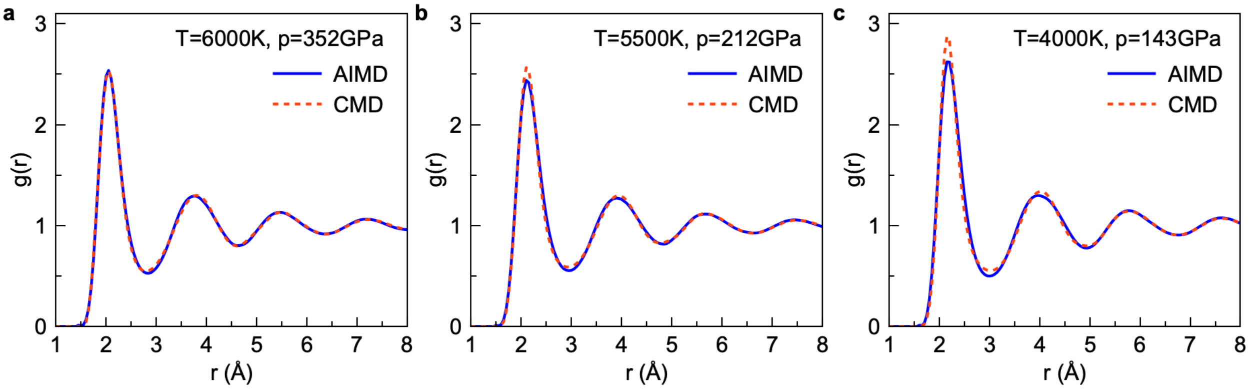


**Figure S1 | Pair correlation functions of liquid Fe under the Earth's core conditions between AIMD and CMD with the present potential.** **a**, T=6000K and p=352GPa. **b**, T=5500K and p=212 GPa. **c**, T=4000K and p=143 GPa.

To test the ability of the developed potential on the predictions of the solidification under the Earth's core conditions, we performed the following test. First, we choose two temperatures for testing: T=4800 K and T=5800 K. Using the developed EAM potential, we created hcp, bcc, and liquid models at these temperatures and p=323 GPa. Then we performed the AIMD NVT simulations using these models, which led to different stresses and pressures, as shown in Table S3. The largest deviations were obtained for the hcp phase at T=4800 K. Such deviations in pressure correspond to about 0.7% for the deviation in the atomic density.

Next, two types of deformation were applied to hcp models to get non-zero $\varepsilon_{xx}$ and $\varepsilon_{zz}$. Only one type of deformation was applied to the bcc models for a non-zero value of $\varepsilon_{xx}$. The

absolute values of $\varepsilon_{\alpha\beta}$ were 0.01. Entire stress tensors were determined from the AIMD simulation for each case. These data allowed us to determine the lattice parameters at the same pressure as was obtained from AIMD simulations for liquid models. New AIMD simulations were performed with these lattice parameters to confirm that all diagonal components of the stress tensors are the same as the liquid pressure and to get the phase energies, allowing us to obtain the latent heats provided in Table S3. The examination of the data presented in Table S3 shows that the developed potential slightly overestimates the c/a ratio for the hcp phase. However, the key property for the simulation of the crystallization is the latent heat and the examination of the data presented in Table S3 shows that the developed potential provides an excellent agreement with the AIMD data.

**Table S3 | Comparison between developed EAM potential and AIMD.**

| Property | AIMD | EAM |
|---|---|---|
| P (liquid at $\rho$=0.1437 atom/Å$^3$ and T=4800 K) (GPa) | 322.6 | 323.0 |
| P (liquid at $\rho$=0.1429 atom/Å$^3$ and T=5800 K) (GPa) | 326.9 | 323.0 |
| $\sigma_{xx}$ (hcp at $\rho$=0.1450 atom/Å$^3$ and T=4800 K) (GPa) | 315.8 | 323.0 |
| $\sigma_{zz}$ (hcp at $\rho$=0.1450 atom/Å$^3$ and T=4800 K) (GPa)[§] | 311.8 | 323.0 |
| $\sigma_{xx}$ (hcp at $\rho$=0.1443 atom/Å$^3$ and T=5800 K) (GPa) | 321.8 | 323.0 |
| $\sigma_{zz}$ (hcp at $\rho$=0.1443 atom/Å$^3$ and T=5800 K) (GPa)[§] | 319.8 | 323.0 |
| p (bcc at $\rho$=0.1451 atom/Å$^3$ and T=4800 K) (GPa) | 323.9 | 323.0 |
| p (bcc at $\rho$=0.1443 atom/Å$^3$ and T=5800 K) (GPa) | 328.7 | 323.0 |
| c/a (hcp at T=4800 K and p≈323 GPa) | 1.622 | 1.629 |
| c/a (hcp at T=5800 K and p≈323 GPa) | 1.624 | 1.628 |
| $\Delta H_m$ (eV/atom) (hcp at T=4800 K and p=323 GPa) | 0.529 | 0.521 |
| $\Delta H_m$ (eV/atom) (hcp at T=5800 K and p=323 GPa) | 0.540 | 0.524 |
| $\Delta H_m$ (eV/atom) (bcc at T=4800 K and p=323 GPa) | 0.365 | 0.367 |
| $\Delta H_m$ (eV/atom) (bcc at T=5800 K and p=323 GPa) | 0.394 | 0.394 |

Finally, we determined the melting temperatures for the hcp and bcc phases at several pressures using the coexistence approach proposed in Ref. [2]. The results are shown in Fig. 1 of the

[§] In the case of the hcp phase the lattice parameters were chosen using the EAM potential which provided $\sigma_{xx}=\sigma_{zz}$; since the AIMD leads to a different c/a ratio, $\sigma_{xx}\neq\sigma_{zz}$ for the same lattice parameters.

main text. Overall, our current melting curve provides the closest agreement to the recent high-pressure experiments for the hcp phases compared to other previous calculated results. Moreover, the developed EAM potential provides the hcp phase as the ground state under the Earth's inner core. It also predicts that the bcc melting temperature is close to the hcp melting temperature at 360 GPa.

Since this potential provides a good melting curve of the hcp phase compared to literature data, a good agreement of elastic constants compared to the AIMD data, and especially excellent agreement for the latent heats, it is suitable for crystallization simulation under the Earth's core conditions.

**Supplementary Note 2 | Kinetic prefactor $\kappa$ in nucleation rate**

From Classical nucleation theory, the nucleation rate, $J$ , can be calculated as $J = \kappa\exp(-\Delta G^*/k_B T)$, where $\Delta G^*$ is the nucleation barrier, $k_B$ is the Boltzmann constant, and $\kappa$ is a kinetic prefactor. The kinetic prefactor $\kappa$ can be derived from the steady-state model [3] as

$$\kappa = \rho_L f^+ \sqrt{\frac{|\Delta\mu|}{6\pi k_B T N^*}}, \quad \text{(S1)}$$

where $f^+$ is the attachment rate of a single atom to the critical nucleus and $\rho_L$ is the liquid density, $\Delta\mu$ is the chemical potential difference between bulk solid and liquid, $N^*$ is the critical nucleus size. As demonstrated by Auer and Frenkel [4], the attachment rate can be computed as the effective diffusion constant for the size change of the critical nucleus as $f^+ = \frac{\langle|\Delta N^*(t)|^2\rangle}{2t}$. Therefore, we employed the iso-configurational ensemble [5] simulation to measure $f^+$ using the critical nucleus obtained from the PEM-MD simulations. In Fig. S2a, 60 independent MD runs starting from the same atomic configuration but with atomic momenta randomly assigned using the Maxwell distribution are shown. The critical nucleus melted in half of the MD runs and grew in the other half runs, which validates the determination of the critical nucleus size. The measured $f^+$ of both hcp and bcc are shown in Fig. S2b. The temperature dependence of obtained $f^+$ can be well fit to the classical kinetic model of atom attachment [3] as

$$f^+ = sN^{*2/3}\frac{6D}{\lambda^2}, \quad \text{(S2)}$$

where $D$ is the liquid diffusivity measured from MD simulation. The hcp nucleus shows a systematically higher attachment rate than that of the bcc nucleus. It should be noted that the effect

of $f^+$ on the nucleation rate is much smaller than the $\Delta G^*$ as $J$ depends exponentially on $\Delta G^*$ in Eq. (S1).

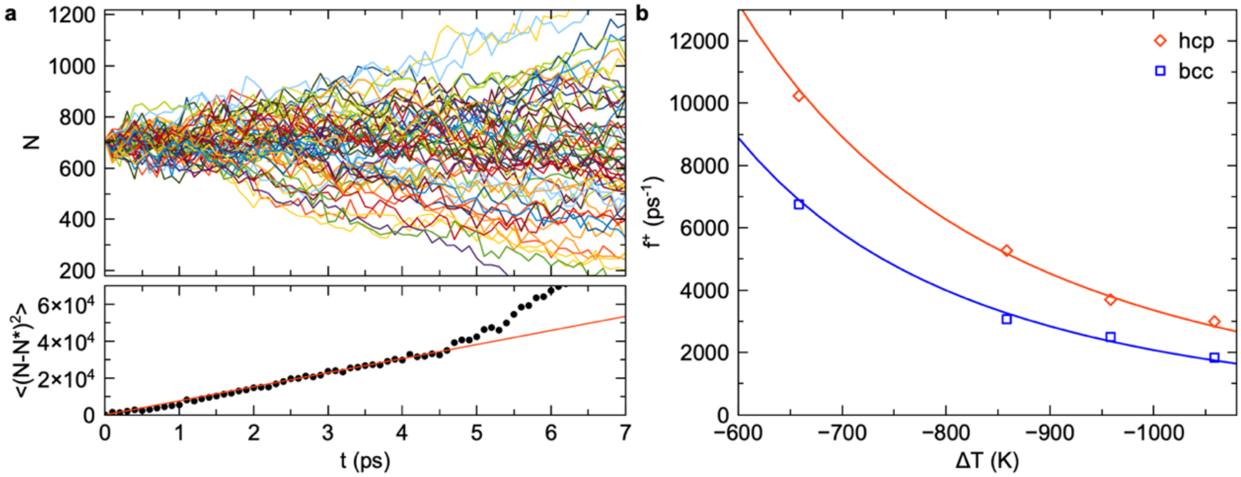


**Figure S2 | Measurement of the attachment rate for the hcp and bcc phases. a**, Iso-configurational ensemble of the hcp critical nucleus obtained at 323 GPa and ΔT=-958K. 60 MD runs are performed starting from the same configuration but with different initial atomic velocities. The bottom panel shows the ensemble average of the nucleus change $\langle|\Delta N^*(t)|^2\rangle = \langle(N(t) - N^*)^2\rangle$. The red line indicates the linear fitting to the first 4 *ps* used to obtain the attachment rate. **b**, The attachment rate as a function of undercooling temperature for the hcp and bcc phases. The symbols are data points obtained from the iso-configurational ensemble averaging. The solid line is fitting to Eqn. (S2)

**Supplementary Note 3 | Effect of input parameters on the waiting time**

To elucidate the effect of the input parameters on the nucleation waiting time of the hcp phase, we substituted the input parameters obtained from the present study with those from Ref. [6]. Figure S3a shows the comparison of the waiting time. It indicates that the different $\Delta\mu$ is the major factor that causes the difference between the current data and the one in [6]. Figure S3b shows the comparison of $\Delta\mu$ obtained in these two works. Using the melting temperature from [6] leads to a decreased $\Delta\mu$. The original $\Delta\mu$ from [6] is even smaller. Because $\Delta\mu$ is essentially correlated with the latent heat based on the Gibbs-Helmholtz equations, these comparisons elucidate the strong effect of the latent heat on the final results. Note that the latent heat provided by the potential developed in the present study is in excellent agreement with the AIMD data as shown in Fig. 1 in the main text.

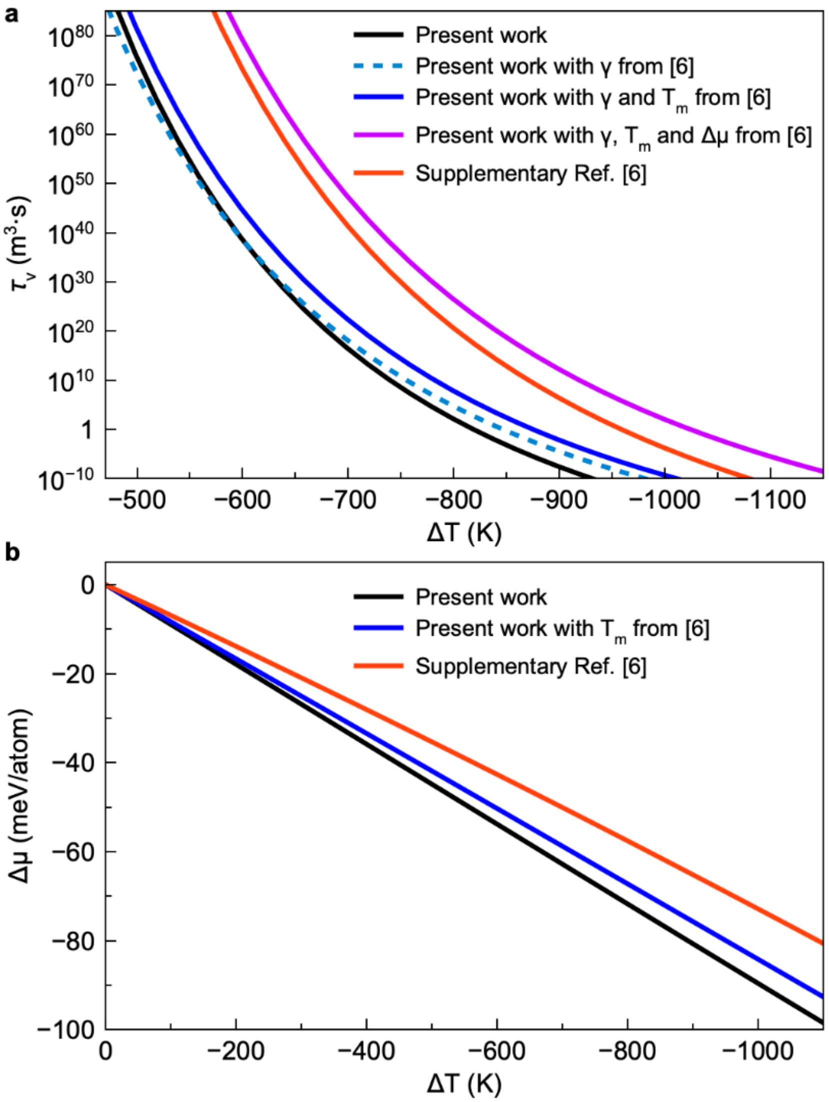


**Figure S3 |** The waiting time and the chemical potential difference for the hcp phase nucleation calculated in the present study and substitution of the current input parameters by those from [6].

**Supplementary Note 4 | Order parameters**

To identify the nucleus type and size in this study, we employ two structural order parameters, bond-orientational order (BOO) parameter [7] and cluster alignment (CA) method [8]. The BOO parameter is based on the correlation between the structures of any two neighbor atoms $i$ and $j$ as $S_{ij} = \sum_{m=-6}^{6} q_{6m}(i) \cdot q_{6m}^{*}(j)$ , where $q_{6m}(i) = \frac{1}{N_b(i)} \sum_{j=1}^{N_b(i)} Y_{lm}(\vec{r}_{ij})$ is the Steinhardt parameter, $Y_{lm}(\vec{r}_{ij})$ are the spherical harmonics, $N_b(i)$ is the number of nearest neighbors of atom $i$ and $\vec{r}_{ij}$ is the vector connecting it with its neighbor $j$. Two neighboring atoms $i$ and $j$ are considered to be connected when $S_{ij}$ exceeds a threshold $S_c$. To choose a reasonable value of $S_c$, an "equal

mislabeling" method [9] was used so that the probability of mislabeling atoms in the bulk liquid as solid-like atoms is the same as the probability of mislabeling atoms in bulk solid as liquid-like atoms. This approach works well when one needs to detect bulk solid atoms within a bulk liquid. However, it tends to mislabel solid atoms at the solid-liquid interface. Therefore it requires another threshold $\xi$ to account for the number of solid-like neighbors. Here the threshold value, $\xi_c$, is chosen to be 6 for the hcp-liquid interfaces and 7 for the bcc-liquid interface. BOO parameter is computed on the fly of PEM-MD to identify the solid-like atoms during the simulation efficiently.

As being demonstrated in [10,11], the nucleus size can be somewhat sensitive to the choice of order parameters. Therefore, in addition to the BOO, CA method [8] was employed to validate the nucleus size by post-processing the simulation trajectory of PEM. The CA method differentiates complex crystal structures by computing the minimal root-mean-square deviation (RMSD) between the atomic cluster and the perfect crystal motifs [12,13]. In Fig. S4, we show the RMSD distributions of atoms in liquid, hcp, and bcc phases under the core conditions. It indicates a good performance of CA on distinguishing the hcp, bcc, and liquid for the present system.

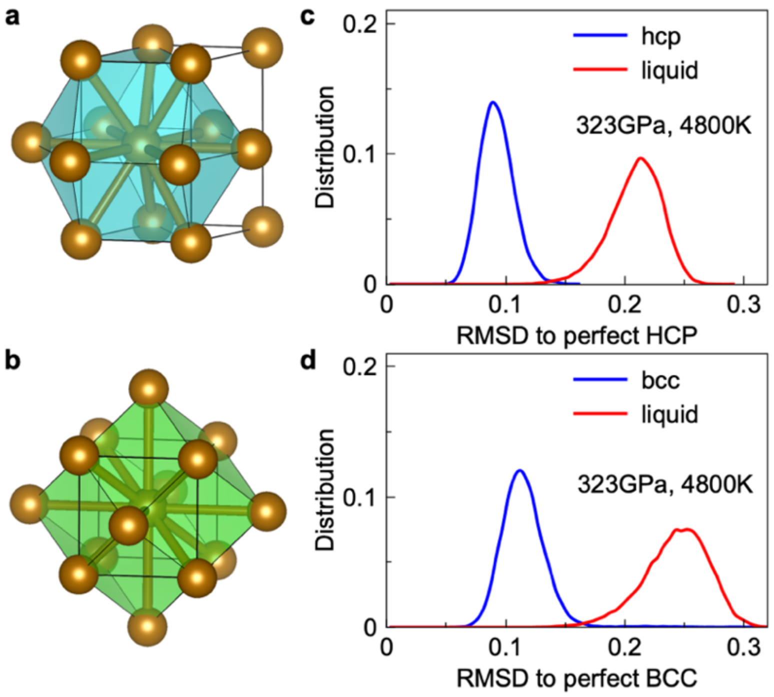


**Figure S4 | Cluster alignment to differentiate the HCP and BCC phases from the liquid. a** and **b** show the hcp and bcc lattices and the clusters (colored polyhedral) used as hcp and bcc templates, respectively. **c** and **d** show the different distribution of root-mean-square deviation (RMSD) of hcp, bcc and liquid.

## Supplementary References


1. Mendelev, M. I. & Srolovitz, D. J. Determination of alloy interatomic potentials from liquid-state diffraction data. *Phys. Rev. B* **66**, 014205 (2002).
2. Morris, J. R., Wang, C. Z., Ho, K. M. & Chan, C. T. Melting line of aluminum from simulations of coexisting phases. *Phys. Rev. B* **49**, 3109–3115 (1994).
3. Kelton, K. F. & Greer, A. L. *Nucleation in condensed matter: application in materials and biology*. (Elsevier, 2010).
4. Auer, S. & Frenkel, D. Numerical prediction of absolute crystallization rates in hard-sphere colloids. *J. Chem. Phys.* **120**, 3015–29 (2004).
5. Widmer-Cooper, A., Harrowell, P. & Fynewever, H. How reproducible are dynamic heterogeneities in a supercooled liquid? *Phys. Rev. Lett.* **93**, 135701 (2004).
6. Davies, C. J., Pozzo, M. & Alfè, D. Assessing the inner core nucleation paradox with atomic-scale simulations. *Earth Planet. Sci. Lett.* **507**, 1–9 (2019).
7. Steinhardt, P. J., Nelson, D. R. & Ronchetti, M. Bond-orientational order in liquids and glasses. *Phys. Rev. B* **28**, 784–805 (1983).
8. Fang, X. W., Wang, C. Z., Yao, Y. X., Ding, Z. J. & Ho, K. M. Atomistic cluster alignment method for local order mining in liquids and glasses. *Phys. Rev. B* **82**, 184204 (2010).
9. Espinosa, J. R., Vega, C., Valeriani, C. & Sanz, E. Seeding approach to crystal nucleation. *J. Chem. Phys.* **144**, 034501 (2016).
10. Zimmermann, N. E. R. *et al.* NaCl nucleation from brine in seeded simulations: Sources of uncertainty in rate estimates. *J. Chem. Phys.* **148**, 222838 (2018).
11. Sun, Y. *et al.* Temperature dependence of the solid-liquid interface free energy of Ni and Al from molecular dynamics simulation of nucleation. *J. Chem. Phys.* **149**, 174501 (2018).
12. Sun, Y. *et al.* ‘Crystal Genes’ in Metallic Liquids and Glasses. *Sci. Rep.* **6**, 23734 (2016).
13. Ren, S. *et al.* Phase Diagram and Structure Map of Binary Nanoparticle Superlattices from a Lennard-Jones Model. *ACS Nano* **14**, 6795–6802 (2020).
